# Supplementary material for: Causally Denoise Word Embeddings Using Half-Sibling Regression
Source: arXiv:1911.10524 source file (2019-11-24)
Supplement: Supplementary file 1 [file Appendix__HSR.pdf]

# Appendix

The Multilayer Perceptrons HSR model (denoted by HSR-MLP) is shown in Algorithm 1. For the hyper-parameters of $MLP()$, we use one hidden layer of size 100 with L2 regularization term $\alpha = 50$.

**Algorithm 1:** HSR-MLP for word vector post-processing

**Input :** (i) $\mathbf{V}^Y$: a $n \times K$ target matrix whose columns are $\{v_i^Y\}_{i=1}^K$, i.e., a collection of off-the-shelf content-word vectors; (ii) $\mathbf{V}^X$: a $n \times P$ input matrix whose columns are $\{v_i^X\}_{i=1}^P$, i.e., a collection of off-the-shelf function-word vectors; (iii) a Multilayer Perceptrons model $MLP()$ with L2 regularization term $\alpha$.

1 **Post-process content-word vectors**:

Step 1.1: *Identify noise contained in content-word vectors*: Train a Multilayer Perceptrons model $MLP^1$ such that

$$\mathbf{V}^Y \approx MLP^1(\mathbf{V}^X).$$

Step 1.2: *Remove noise contained in content-word vectors*:

$$\hat{\mathbf{V}}^Y := \mathbf{V}^Y - MLP^1(\mathbf{V}^X).$$

2 **Post-process stop-word vectors**:

Step 2.1: *Identify noise contained in stop-word vectors*: Train a Multilayer Perceptrons model $MLP^2$ such that

$$\mathbf{V}^X \approx MLP^2(\mathbf{V}^Y).$$

Step 2.2: *Remove noise contained in stop-word vectors*:

$$\hat{\mathbf{V}}^X := \mathbf{V}^X - MLP^2(\mathbf{V}^Y).$$

**Output:** (i) HSR-MLP post-processed content-word vectors $\{\hat{v}_i^Y\}$, which are columns of the matrix $\hat{\mathbf{V}}^Y$; (ii) HSR-MLP post-processed stop-word vectors $\{\hat{v}_i^X\}$, which are columns of the matrix $\hat{\mathbf{V}}^X$.

Next, we present the detailed experimental results of Half-Sibling Regression using both Ridge Regression (denoted by HSR-RR) and Multilayer Perceptrons (denoted by HSR-MLP). Table 1 reports the Spearman's rank correlation coefficient of the seven word similarity tasks, in which the result marked in bold is the best, and the results underlined are the top three results. Table 2 shows the Pearson correlation coefficient of 20 semantic textual similarity tasks. Table 3 reports the five-fold cross-validation accuracy of four sentiment analysis tasks.

Table 1: Spearman's rank correlation coefficient of seven word similarity tasks

| | WORD2VEC | | | | | | GLOVE | | | | | | PARAGRAM | | | | | |
|---|---|---|---|---|---|---|---|---|---|---|---|---|---|---|---|---|---|---|
| | Orig. | ABTT | CN | SB | HSR-RR | HSR-MLP | Orig. | ABTT | CN | SB | HSR-RR | HSR-MLP | Orig. | ABTT | CN | SB | HSR-RR | HSR-MLP |
| **RG65** | 0.7494 | 0.7869 | **0.8041** | 0.7964 | 0.7569 | 0.7504 | 0.7603 | 0.7648 | **0.7913** | 0.7850 | 0.7694 | 0.7604 | 0.7630 | 0.7683 | 0.7594 | **0.7898** | 0.7760 | 0.7655 |
| **WordSim-353** | 0.6999 | 0.6929 | 0.6992 | 0.6856 | **0.7059** | 0.7002 | 0.7379 | 0.7668 | 0.7886 | 0.7115 | **0.7887** | 0.7761 | 0.7302 | **0.7386** | 0.7321 | 0.7196 | 0.7338 | 0.7337 |
| **RW** | 0.5997 | 0.5984 | 0.6036 | 0.5998 | 0.6033 | **0.6039** | 0.5101 | 0.5716 | **0.5898** | 0.4879 | 0.5580 | 0.5589 | 0.5972 | **0.6038** | 0.6006 | 0.5769 | 0.6023 | 0.6020 |
| **MEN** | 0.7706 | **0.7929** | 0.7901 | 0.7888 | 0.7726 | 0.7712 | 0.8013 | 0.8234 | **0.8339** | 0.7853 | 0.8258 | 0.8193 | 0.7728 | 0.7705 | 0.7746 | 0.7693 | **0.7750** | 0.7726 |
| **MTurk** | 0.6831 | 0.6538 | 0.6610 | 0.6846 | 0.6854 | **0.6881** | 0.6916 | **0.7233** | 0.7116 | 0.6731 | 0.7074 | 0.7105 | 0.6300 | 0.6106 | 0.6251 | 0.6147 | **0.6319** | 0.6313 |
| **SimLex-999** | 0.4427 | 0.4629 | **0.4728** | 0.4702 | 0.4672 | 0.4623 | 0.4076 | 0.4650 | **0.4858** | 0.3985 | 0.4728 | 0.4625 | 0.6847 | 0.6862 | 0.6854 | 0.6878 | **0.6903** | 0.6876 |
| **SimVerb-3500** | 0.3659 | 0.3792 | 0.3868 | 0.3865 | **0.3978** | 0.3950 | 0.2842 | 0.3433 | 0.3632 | 0.2671 | **0.3980** | 0.3679 | 0.5411 | 0.5461 | 0.5413 | 0.5389 | **0.5518** | 0.5439 |

Table 2: Pearson correlation coefficient of 20 semantic textual similarity tasks

| | WORD2VEC | | | | | | GLOVE | | | | | | PARAGRAM | | | | | |
|---|---|---|---|---|---|---|---|---|---|---|---|---|---|---|---|---|---|---|
| | Orig. | ABTT | CN | SB | HSR-RR | HSR-MLP | Orig. | ABTT | CN | SB | HSR-RR | HSR-MLP | Orig. | ABTT | CN | SB | HSR-RR | HSR-MLP |
| **STS-2012-MSRpar** | **41.78** | 38.70 | 39.42 | 40.77 | 34.42 | 38.27 | **42.06** | 41.41 | 41.27 | 41.15 | 32.49 | 35.01 | 39.32 | 38.84 | 39.84 | 37.72 | **41.44** | 39.34 |
| **STS-2012-MSRvid** | 76.27 | 75.60 | 75.32 | 74.98 | **79.63** | 77.05 | 65.85 | 67.84 | 62.50 | 64.71 | **80.03** | 69.71 | 56.34 | 57.65 | 56.78 | 55.55 | **62.31** | 56.02 |
| **STS-2012-surprise.OnWN** | 70.62 | 70.89 | 70.73 | 69.99 | 71.27 | **71.54** | 60.74 | 69.48 | 67.87 | 57.02 | **72.24** | 70.51 | 62.60 | 64.61 | 63.21 | 60.68 | **67.91** | 63.35 |
| **STS-2012-SMTeuroparl** | 31.20 | 35.71 | 35.29 | 33.88 | **40.32** | 36.97 | 51.97 | **54.36** | 52.58 | 50.06 | 51.60 | 50.87 | 50.64 | 51.64 | 50.63 | 51.34 | **51.92** | 50.27 |
| **STS-2012-surprise.SMTnews** | **51.07** | 46.24 | 47.34 | 47.10 | 50.09 | 49.40 | 46.35 | 48.19 | 47.69 | 45.18 | **54.41** | 54.02 | 52.94 | 50.18 | 52.66 | **54.16** | 53.87 | 51.47 |
| **STS-2012** | 54.19 | 53.43 | 53.62 | 53.34 | **55.15** | 54.65 | 53.39 | 56.26 | 54.38 | 51.62 | **58.15** | 56.02 | 52.37 | 52.58 | 52.62 | 51.89 | **55.49** | 52.09 |
| **STS-2013-FNWN** | 39.68 | 43.51 | 43.40 | 42.95 | **49.09** | 45.82 | 39.48 | 45.81 | 42.03 | 39.15 | **46.47** | 36.91 | 35.79 | 36.05 | 35.93 | 34.35 | **38.00** | 35.42 |
| **STS-2013-OnWN** | 67.98 | 70.56 | 69.29 | 69.12 | **75.57** | 73.36 | 53.75 | 63.86 | 57.45 | 52.36 | **74.91** | 68.56 | 48.07 | 48.18 | 48.23 | 48.28 | **56.57** | 48.88 |
| **STS-2013-headlines** | 63.29 | 63.24 | 63.62 | 63.22 | **63.65** | 63.55 | 63.54 | 66.70 | 67.00 | 60.65 | **68.56** | 67.46 | 64.43 | 65.13 | 64.69 | 62.99 | **66.90** | 64.64 |
| **STS-2013** | 56.98 | 59.10 | 58.77 | 58.43 | **62.77** | 60.91 | 52.26 | 58.79 | 55.49 | 50.72 | **63.31** | 57.64 | 49.43 | 49.79 | 49.62 | 48.54 | **53.82** | 49.65 |
| **STS-2014-OnWN** | 74.85 | 75.92 | 75.27 | 74.43 | **81.40** | 78.70 | 61.91 | 70.93 | 66.43 | 60.36 | **81.39** | 75.28 | 60.29 | 61.95 | 60.75 | 59.45 | **68.30** | 61.13 |
| **STS-2014-deft-forum** | 41.30 | 42.25 | 42.74 | 42.03 | **46.73** | 45.11 | 28.82 | 38.90 | 37.57 | 25.91 | **45.85** | 42.36 | 35.17 | 37.60 | 35.75 | 33.59 | **40.84** | 35.90 |
| **STS-2014-deft-news** | 66.76 | 64.87 | 65.45 | 64.97 | **67.88** | 66.94 | 63.41 | 68.72 | 69.08 | 61.27 | **70.60** | 70.00 | 62.19 | 63.73 | 62.75 | 61.09 | **66.66** | 62.11 |
| **STS-2014-headlines** | 60.87 | 60.61 | **61.09** | 60.66 | 60.93 | 60.70 | 59.28 | 61.34 | 61.71 | 56.25 | **64.01** | 62.44 | 60.84 | 60.72 | 60.97 | 60.21 | **62.83** | 60.83 |
| **STS-2014-tweet-news** | 73.33 | 75.13 | 74.87 | 73.66 | 76.00 | **76.04** | 62.43 | 74.62 | 75.38 | 58.70 | 75.09 | **76.62** | 69.29 | 72.43 | 70.14 | 66.75 | **75.16** | 70.18 |
| **STS-2014-images** | 77.44 | 77.81 | 78.42 | 77.11 | **80.55** | 78.99 | 61.89 | 69.40 | 65.81 | 59.03 | **78.45** | 72.74 | 53.67 | 58.29 | 54.86 | 51.58 | **65.10** | 53.72 |
| **STS-2014** | 65.76 | 66.10 | 66.31 | 65.48 | **68.92** | 67.75 | 56.29 | 63.99 | 62.66 | 53.59 | **69.23** | 66.57 | 56.91 | 59.12 | 57.54 | 55.45 | **63.15** | 57.31 |
| **STS-2015-answers-forums** | 52.65 | 54.01 | 53.99 | 50.51 | **66.77** | 60.41 | 36.86 | 49.58 | 48.62 | 36.76 | **65.46** | 61.10 | 38.79 | 41.19 | 39.25 | 38.35 | **48.37** | 38.98 |
| **STS-2015-answers-students** | 70.82 | 70.92 | 71.65 | 69.74 | **72.16** | 71.90 | 62.77 | 69.46 | 69.68 | 61.84 | 67.38 | **70.06** | 67.52 | 69.46 | 67.96 | 66.80 | **71.98** | 67.39 |
| **STS-2015-belief** | 60.11 | 61.91 | 61.62 | 58.10 | **77.08** | 69.41 | 44.20 | 61.43 | 59.77 | 41.19 | **76.12** | 73.94 | 49.77 | 55.57 | 50.79 | 46.98 | **61.32** | 51.32 |
| **STS-2015-headlines** | 68.11 | 68.28 | 68.65 | 68.19 | **69.02** | 68.42 | 65.42 | 68.90 | 69.20 | 63.25 | **71.41** | 69.71 | 67.85 | 68.40 | 68.09 | 66.92 | **70.38** | 67.99 |
| **STS-2015-images** | 80.07 | 80.18 | 80.74 | 79.48 | **83.08** | 81.78 | 69.14 | 73.53 | 71.43 | 67.81 | **80.58** | 74.86 | 66.55 | 68.29 | 67.08 | 65.55 | **73.17** | 65.96 |
| **STS-2015** | 66.35 | 67.06 | 67.33 | 65.20 | **73.62** | 70.38 | 55.68 | 64.58 | 63.74 | 54.17 | **72.19** | 69.93 | 58.10 | 60.58 | 58.63 | 56.92 | **65.04** | 58.33 |
| **SICK** | 72.25 | **72.49** | 72.40 | 72.32 | 72.02 | 72.48 | 66.64 | 68.12 | 66.42 | 66.03 | **71.62** | 67.85 | 64.55 | 64.89 | 64.78 | 64.05 | **67.07** | 64.24 |

Table 3: Five-fold cross-validation accuracy of four sentiment analysis tasks

| | WORD2VEC | | | | | | GLOVE | | | | | | PARAGRAM | | | | | |
|---|---|---|---|---|---|---|---|---|---|---|---|---|---|---|---|---|---|---|
| | Orig. | CN | ABTT | SB | HSR-RR | HSR-MLP | Orig. | CN | ABTT | SB | HSR-RR | HSR-MLP | Orig. | CN | ABTT | SB | HSR-RR | HSR-MLP |
| **AR** | 0.8375 | 0.8338 | 0.8329 | 0.8302 | 0.8377 | **0.8380** | 0.8441 | 0.8431 | 0.8444 | 0.8426 | **0.8454** | 0.8436 | 0.8124 | 0.8129 | 0.8113 | 0.8124 | **0.8152** | 0.8120 |
| **CR** | 0.7800 | 0.7792 | 0.7718 | 0.7726 | **0.7824** | 0.7800 | **0.7829** | 0.7800 | 0.7808 | 0.7819 | 0.7792 | 0.7787 | 0.7657 | 0.7649 | 0.7628 | 0.7644 | **0.7673** | 0.7670 |
| **IMDB** | 0.8392 | 0.8369 | 0.8370 | 0.8281 | **0.8434** | 0.8394 | 0.8491 | 0.8453 | **0.8493** | 0.8459 | **0.8493** | 0.8482 | 0.7957 | 0.7960 | 0.7953 | 0.7938 | **0.7999** | 0.7950 |
| **STS-B** | 0.8071 | 0.8062 | 0.8048 | 0.8052 | 0.8056 | **0.8083** | 0.8044 | 0.8045 | 0.8049 | 0.8031 | **0.8053** | 0.8035 | 0.7818 | 0.7819 | 0.7778 | 0.7813 | **0.7846** | 0.7833 |
